# Supplementary material for: Students Success Modeling: Most Important Factors
Source: arXiv:2309.13052 source file (2023-09-06)
Supplement: Supplementary file 1 [file Appendix.tex]

\begin{table}
\caption{Features Descriptions}
\label{table}
\setlength{\tabcolsep}{3pt}
\begin{tabular}{|p{75pt}|p{215pt}|}
\hline
Feature Name& 
Description& 
\hline
A01&ACT ENGLISH\\
A02&ACT MATH\\
A03&ACT READING\\
A04&ACT SCIENCE REASONING\\
A05&ACT COMPOSITE\\
ACCM&ACCUPLACER CLASSIC ELEM. ALG.\\
ACCNGM&NEXT GEN ACCU QR/ALG/STATS\\
ACCNGR&NEXT GEN ACCU READING\\
ACCR&ACCUPLACERCLASSIC READINGCOMP\\
ACCW&ACCUPLACER WRITEPLACER\\
Aids&Indicate the total financial aid students used\\
AT-RISK-HOMELESS&Indicate whether student is at the risk of being homeless\\
Avg-Points&Average points student got in each semester from online classes\\
Avg-Points-perClass&Average points student got in each semester from each online class\\
Avg-Weighted&Average weighted points student got in each semester from online classes\\
Avg-Weighted-perClass&Average weighted points student got in each semester from each online class\\
COME&"Indicate the ""Compass Writing"" grade"\\
COMG&"Indicate the ""Compass Geometry"" grade"\\
COMM&"Indicate the ""Compass  Algebra"" grade"\\
COMR&"Indicate the ""Compass Reading"" grade"\\
CROW-DISTANCE&indicate CROW distance\\
DEPEND-AGE-0-5&Indicate the number of student's dependence (age less than 5)\\
DEPEND-AGE-13-PLUS&Indicate the number of student's dependence (age greater than 13 )\\
DEPEND-AGE-6-12&Indicate the number of student's dependence (age between 6 and 12)\\
DRIVE-DISTANCE&indicate driving distance from living place to school\\
DRIVE-DURATION&Indicate driving  time from living place to school\\
FAM-MEMB&The number of people in the student's household during the school year.\\
Father-EDU-Status-Changed&Indicate if the father's education status changed?\\
FATHER-HIGHEST-GRADE&student's father's education status\\
FOOD-STAMPS&Indicate if student used the food stamp\\
GPA&The student GPA for the current semester\\
Grants&Total grant amounts\\
HAS-LEGAL-DEPEND&Indicates whether the student has legal dependents other than a spouse for determining dependency status.\\
HOURS-ATTEMPTED&Hours student attampted in the current semester\\
HOURS-EARNED&Hours student earned in the current semester\\
House&Indicate if the student owns a house\\
HS-GPA&High School GPA\\
I-GPA&Institute GPA\\
I-HOURS-ATTEMPTED&Institute hours student attampted in the current semester\\
I-HOURS-EARNED&Institute hours student earned in the current semester\\
I-QUALITY-POINTS&Institute quality point in the current semester\\
Loans&Total amounts of loan student got\\
LSE&Learning Support English Grade\\
LSM1&Learning Support MATH 1 Grade\\
LSM2&Learning Support MATH 2 Geade\\
Meal&Indicate if the student used the meal plan\\
Mother-EDU-Status-Changed&Indicate if the mother's education status changed?\\
MOTHER-HIGHEST-GRADE&Student's mother's education status\\
No-ForumId&Number of forum student participated in \\
NO-IN-COLL&total number of family members in the student's household that will attend college at least half-time.\\
indicate &The number of post student sent per semster\\
No-Session&Indicate the total session time\\
No-Submission&Indicate the total number of assignment submition\\
No-TopicId&Indicate the total number of topic student participated in\\
Paid By Student&Indicate the total amount which student paid from his/her tuition \\
PAR-FAM-MEMB&The number of family members in the parent's household.\\
PAR-FOOD-STAMPS&Indicates whether anyone in the parents' household received Supplemental Nutrition Assistance Program (SNAP) benefits.\\
PAR-MRTL-STATUS&The marital status of the student's parents.\\
PAR-NO-IN-COLL&The number of people in the parent's household that will be enrolled in college at least half-time.\\
PAR-RECD-SSI&Indicates whether the applicant's parents received Supplemental Security Income.\\
PAR-RECD-TANF&Indicates whether the applicant's parents received Temporary Assistance for Needy Families.\\
PAR-RECD-WIC&"ndicates whether anyone in the applicant's parents' household received assistance from the Women Infants and Children Program."\\
PAR-SCHOOL-LUNCH&Indicates whether anyone in the applicant's parents' household received Free or Reduced Price School Lunch benefits.\\
Parking&Indicate if the student used parking?\\
PELL&Total amounts of PELL student got\\
QUALITY-POINTS&Quality point per semester\\
RECD-SSI&RECD-SSI\\
RECD-TANF&RECD-TANF\\
RECD-WIC&RECD-WIC\\
S01&SAT CRITICAL READING\\
S02&SAT MATHEMATICS\\
S05&SAT TSWE SCORE\\
S07&SAT WRITING\\
SPS-INC-FR-WRK&he amount of income earned from work by the student's spouse in the base year.\\
SS01&SELF REPORTED SAT VERBAL\\
SS02&SELF REPORTED SAT MATH\\
SS07&SELF REPORTED SAT WRITING\\
Sum-AttemptNumber&Total number of quiz attempts\\
Sum-NumViews&Total number of course material views\\
Sum-SessionSecond&Total session time\\
T-GPA&Transferred GPA\\
T-HOURS-ATTEMPTED&Transferred hours student attempted in the current semester\\
T-HOURS-EARNED&Transferred hours student earned in the current semester\\
T-QUALITY-POINTS&Transferred quality points student earned in the current semester\\
TOT-FAM-CTRB&The total family contribution for the primary institution calculation.\\
TOT-SAR-EFC&what the SAR EFC was for a person when they were added in data load.\\
Tuition-Fee&The total amount of Tuition fee for the semester\\
US-VET&Indicates if the student is a veteran of the US Armed Forces.\\
Visit-AvglTime-Class&Average visit time for class material \\
Visit-TotalTime-user&Total visit time for class material \\
WARD-OF-COURT&Indicates if the student reported being a ward of the court or is an orphan.\\

\hline
\end{tabular}
\label{tab1}
\end{table}
